# Supplementary material for: Understanding Graph Neural Networks from Graph Signal Denoising Perspectives
Source: arXiv:2006.04386 source file (2020-06-08)
Supplement: Supplementary file 1 [file appendix.pdf]

## 1 A Background

2 In this section, we introduce the background of graph signal denoising, spectral graph convolutions,  
3 and graph attentions.

### 4 A.1 Graph Signal Denoising

5 Given a graph  $\mathcal{G} = (\mathcal{V}, \mathbf{A})$  with noisy node features  $\mathbf{X}$ , and assume that the ground-truth node  
6 features, denoted as  $\hat{\mathbf{X}}$ , are smooth, graph signal denoising (GSD) (Berger et al., 2017; Chen et al.,  
7 2015) aims to recover smooth graph signals  $\hat{\mathbf{X}}$  from noisy input node features  $\mathbf{X}$ . The GSD problem  
8 of a noisy graph can be formulated as an optimization problem that aims to obtain the smoothest  
9 node features subject to the effect of noise in the graph.

### 10 A.2 Spectral Graph Convolutions

11 SGCNs were mainly inspired by graph signal processing (GSP). In the field of GSP, the *graph Fourier*  
12 *transform* (Hammond et al., 2011; Sandryhaila & Moura, 2013) of  $\mathbf{x}$  is defined as  $\bar{\mathbf{x}} = \mathbf{U}^\top \mathbf{x}$  and the  
13 *inverse* graph Fourier transform is defined as  $\mathbf{x} = \mathbf{U} \bar{\mathbf{x}}$ . Then, the spectral graph convolution of the  
14 input signal  $\mathbf{x}$  with a filter  $\mathbf{g}_\theta = \text{diag}(\theta)$  parameterized by  $\theta \in \mathbb{R}^N$  in the Fourier domain (Henaff  
15 et al., 2015) is defined as

$$\mathbf{g}_\theta \star \mathbf{x} = \mathbf{U} \mathbf{g}_\theta \mathbf{U}^\top \mathbf{x}, \quad (12)$$

16 where  $\star$  denotes the convolution operation. ChebyNet (Defferrard et al., 2016) uses  $K$ -order Cheby-  
17 shev polynomials to approximate the filter  $\mathbf{g}_\theta$  and obtains a new convolution:

$$\mathbf{g}_{\text{ChebyNet}} \star \mathbf{x} = \sum_{k=0}^K \theta_k T_k(\tilde{\mathbf{L}}_n) \mathbf{x}, \quad (13)$$

18 where  $T_k(x) = 2xT_{k-1}(x) - T_{k-2}(x)$ ,  $T_0(x) = 1$  and  $T_1(x) = x$ ,  $\tilde{\mathbf{L}}_n = \frac{2}{\lambda_{\max}} \mathbf{L}_n - \mathbf{I}_N$ , and  
19  $\theta$  is a vector of Chebyshev coefficients. GCN (Kipf & Welling, 2017) introduces a first-order  
20 approximation of ChebyNet using  $K = 1$  and  $\lambda_{\max} = 2$  and the renormalization trick  $\mathbf{I}_N + \mathbf{A}_n \rightarrow$   
21  $\tilde{\mathbf{D}}^{-1/2}(\mathbf{I}_N + \mathbf{A})\tilde{\mathbf{D}}^{-1/2} = \tilde{\mathbf{D}}^{-1/2} \tilde{\mathbf{A}} \tilde{\mathbf{D}}^{-1/2}$ . The resulting graph convolution becomes

$$\mathbf{g}_{\text{GCN}} \star \mathbf{x} = \tilde{\mathbf{A}}_n \mathbf{x}, \quad (14)$$

22 where  $\tilde{\mathbf{A}}_n = \tilde{\mathbf{D}}^{-1/2} \tilde{\mathbf{A}} \tilde{\mathbf{D}}^{-1/2}$ ,  $\tilde{\mathbf{D}} = \text{diag}(\tilde{d}_1, \dots, \tilde{d}_N)$ , and  $\tilde{d}_i = \sum_{j=1}^N \tilde{A}_{ij}$ . SGC (Wu et al., 2019)  
23 successively removes nonlinearities and collapses the weight matrices between  $K$  consecutive layers  
24 of GCN and further simplifies the convolution as

$$\mathbf{g}_{\text{SGC}} \star \mathbf{x} = \tilde{\mathbf{A}}_n^K \mathbf{x}. \quad (15)$$

### 25 A.3 Graph Attentions

26 Unlike SGCN, GANNs were mainly motivated by attention mechanisms in computer vision. GANNs  
27 suggest that the contributions of neighboring nodes to the central node are different during the  
28 aggregation. Here, we discuss two representative GANN models, GAT (Velickovic et al., 2018)  
29 and AGNN (Thekumparampil et al., 2018). GAT utilizes a graph attention mechanism to learn the  
30 aggregation strengths between two connected nodes in each layer. Let  $\mathbf{H}^{(t)}$  be the  $t$ -th layer output  
31 of a neural network, the graph attention mechanism of GAT is defined as

$$a_{ij}^{(t)} = \text{softmax} \left( f(\mathbf{a}^\top [\mathbf{W} \mathbf{H}_i^{(t)} \parallel \mathbf{W} \mathbf{H}_j^{(t)}])_{j \in \mathcal{N}_i \cup \{i\}} \right), \quad (16)$$

32 where  $f(\cdot)$  is the LeakyReLU function, the matrix  $\mathbf{W}$  and the vector  $\mathbf{a}$  are learnable parameters.  
33 Then, GAT aggregates neighborhood information in terms of the learned attention coefficients:

$$\mathbf{H}_i^{(t+1)} = \sigma \left( \sum_{j \in \mathcal{N}_i \cup \{i\}} a_{ij}^{(t)} \mathbf{W} \mathbf{H}_j^{(t)} \right), \quad (17)$$

where  $\mathbf{H}^{(0)} = \mathbf{X}$  and  $\sigma(\cdot)$  is the activation function. AGNN defines the graph attention mechanism in terms of the cosine similarity of node embeddings between connected nodes:

$$a_{ij}^{(t)} = \text{softmax} \left( \left[ \beta \frac{\mathbf{H}_i^{(t)\top} \mathbf{H}_j^{(t)}}{\|\mathbf{H}_i^{(t)}\| \|\mathbf{H}_j^{(t)}\|} \right]_{j \in \mathcal{N}_i \cup \{i\}} \right), \quad (18)$$

where  $\mathbf{H}^{(0)} = \text{ReLU}(\mathbf{X}\mathbf{W})$  and  $\beta$  is a learnable parameter. Similarly, AGNN aggregates neighborhood information by

$$\mathbf{H}_i^{(t+1)} = \sum_{j \in \mathcal{N}_i \cup \{i\}} a_{ij}^{(t)} \mathbf{H}_j^{(t)}. \quad (19)$$

## B Theorem

### B.1 Proof of Proposition 1

*Proof.* For ChebyNet, by Eq.13 we have

$$\begin{aligned} \sum_{k=0}^K \theta_k T_k(\tilde{\mathbf{L}}_n) &= \theta_0 T_0(\tilde{\mathbf{L}}_n) + \theta_1 T_1(\tilde{\mathbf{L}}_n) + \theta_2 T_2(\tilde{\mathbf{L}}_n) + \cdots + \theta_K T_K(\tilde{\mathbf{L}}_n) \\ &= \theta_0 \mathbf{I}_N + \theta_1 \tilde{\mathbf{L}}_n + \theta_2 (2\tilde{\mathbf{L}}_n^2 - \mathbf{I}_N) + \cdots + \theta_K (2\tilde{\mathbf{L}}_n T_{K-1}(\tilde{\mathbf{L}}_n) - T_{K-2}(\tilde{\mathbf{L}}_n)) \\ &\stackrel{(a)}{=} \theta'_0 \mathbf{I}_N + \theta'_1 \tilde{\mathbf{L}}_n + \theta'_2 \tilde{\mathbf{L}}_n^2 + \cdots + \theta'_K \tilde{\mathbf{L}}_n^K \\ &= \theta'_0 \mathbf{I}_N + \theta'_1 \left( \frac{2}{\lambda_{\max}} \mathbf{L}_n - \mathbf{I}_N \right) + \theta'_2 \left( \frac{2}{\lambda_{\max}} \mathbf{L}_n - \mathbf{I}_N \right)^2 + \cdots + \theta'_K \left( \frac{2}{\lambda_{\max}} \mathbf{L}_n - \mathbf{I}_N \right)^K \\ &\stackrel{(a)}{=} \theta''_0 \mathbf{I}_N + \theta''_1 \mathbf{A}_n + \theta''_2 \mathbf{A}_n^2 + \cdots + \theta''_K \mathbf{A}_n^K. \end{aligned} \quad (20)$$

where  $\stackrel{(a)}{=}$  indicates that we re-parametrize the coefficients. Eq.4 and Eq.20 show that the result of ChebyNet graph convolution on node features  $\mathbf{X}$  is a  $K$ -order polynomial approximation of  $\hat{\mathbf{X}}^*$ .

For SGC, when  $K \geq 2$ , by Eq.15 we have:

$$\begin{aligned} \tilde{\mathbf{A}}^K &= \left( \tilde{\mathbf{D}}^{-\frac{1}{2}} (\mathbf{I}_N + \mathbf{A}) \tilde{\mathbf{D}}^{-\frac{1}{2}} \right)^K \\ &= \left( \tilde{\mathbf{D}}^{-1} + \tilde{\mathbf{D}}^{-\frac{1}{2}} \mathbf{A} \tilde{\mathbf{D}}^{-\frac{1}{2}} \right)^K \\ &\approx \left( \tilde{\mathbf{D}}^{-1} + \mathbf{D}_r \mathbf{A}_n \right)^K \\ &= \tilde{\mathbf{D}}^{-K} + K \tilde{\mathbf{D}}^{-1} \mathbf{D}_r \mathbf{A}_n + \frac{K(K-1)}{2!} (\tilde{\mathbf{D}}^{-1} \mathbf{D}_r)^2 \mathbf{A}_n^2 + \frac{K(K-1)(K-2)}{3!} (\tilde{\mathbf{D}}^{-1} \mathbf{D}_r)^3 \mathbf{A}_n^3 \\ &\quad + \cdots + (\tilde{\mathbf{D}}^{-1} \mathbf{D}_r)^K \mathbf{A}_n^K, \end{aligned} \quad (21)$$

where  $\mathbf{D}_r = \text{diag}(d_1/\tilde{d}_1, \dots, d_N/\tilde{d}_N)$  and  $d_i/\tilde{d}_i \leq 1$ . Therefore, by Eq.4 and Eq.21 the result of SGC on node features is a  $K$ -order polynomial approximation of  $\hat{\mathbf{X}}^*$ . Note that GSDN-F and SGC are somewhat similar in the form of approximating the optimal solution of Problem 1. However, the approximation of GSDN-F is better than that of SGC. The reason is that SGC does not well approximate the coefficients of the Taylor expansion of the optimal solution. In contrast, GSDN-F directly uses the Taylor expansion of the optimal solution as its convolution kernel and thus the gap between the results of GSDN-F and the optimal solution should be smaller than the gap between the results of SGC and the optimal solution. SGC can be viewed as a degenerate form of GSDN-F.

For GCN,  $K = 1$ . Then  $\tilde{\mathbf{A}} \approx \tilde{\mathbf{D}}^{-1} + \mathbf{D}_r \mathbf{A}_n$ . Therefore, the result of GCN on node features is a first-order polynomial approximation of  $\hat{\mathbf{X}}^*$ .  $\square$

54 **B.2 Proof of Proposition 3**

55 *Proof.* Let  $\mathbf{H} = (1 - \alpha) \sum_{k=0}^K (\alpha \mathbf{A}_n)^k$ , when  $0 \leq \alpha < 1$  and  $K$  is large, we obtain:

$$\begin{aligned}
 \mathbf{H} &= (1 - \alpha) \sum_{k=0}^K (\alpha \mathbf{A}_n)^k \\
 &= (1 - \alpha) \sum_{k=0}^K (\alpha \mathbf{Q} \mathbf{\Omega} \mathbf{Q}^\top)^k \\
 &= (1 - \alpha) \mathbf{Q} \begin{bmatrix} \frac{1 - (\alpha \omega_1)^K}{1 - \alpha \omega_1} & & \\ & \ddots & \\ & & \frac{1 - (\alpha \omega_N)^K}{1 - \alpha \omega_N} \end{bmatrix} \mathbf{Q}^\top \\
 &\approx (1 - \alpha) \mathbf{Q} \begin{bmatrix} \frac{1}{1 - \alpha \omega_1} & & \\ & \ddots & \\ & & \frac{1}{1 - \alpha \omega_N} \end{bmatrix} \mathbf{Q}^\top \\
 &= \mathbf{Q} \begin{bmatrix} 1 - \frac{1 - \omega_1}{\frac{1}{\alpha} - \omega_1} & & \\ & \ddots & \\ & & 1 - \frac{1 - \omega_N}{\frac{1}{\alpha} - \omega_N} \end{bmatrix} \mathbf{Q}^\top. \tag{22}
 \end{aligned}$$

56 where  $\mathbf{A}_n = \mathbf{Q} \mathbf{\Omega} \mathbf{Q}^\top$  is the eigen-decomposition of  $\mathbf{A}_n$ ,  $\mathbf{Q}$  is the matrix of eigenvectors of  $\mathbf{A}_n$ ,  $\mathbf{\Omega}$  is  
 57 its diagonal matrix of eigenvalues and  $0 \leq \omega_1 \leq \omega_2 \leq \dots \leq \omega_N \leq 1$  are the eigenvalues. Then we  
 58 have:

$$\begin{aligned}
 \mathbf{Var}(\hat{\mathbf{x}}^* | \alpha) &= \mathbb{E} [||\hat{\mathbf{x}}^* - \mathbb{E}[\hat{\mathbf{x}}^*]||_2^2] \\
 &= \mathbb{E} [||\mathbf{H}\mathbf{x} - \mathbf{H}\hat{\mathbf{x}}||_2^2] \\
 &= \mathbb{E} [||\mathbf{H}\mathbf{z}||_2^2] \\
 &= \mathbf{Tr}(\mathbf{H}^2 \mathbf{\Sigma}) \\
 &\approx \mathbf{Tr} \left( \mathbf{Q} \begin{bmatrix} 1 - \frac{1 - \omega_1}{\frac{1}{\alpha} - \omega_1} & & \\ & \ddots & \\ & & 1 - \frac{1 - \omega_N}{\frac{1}{\alpha} - \omega_N} \end{bmatrix} \mathbf{Q}^\top \right)^2 \mathbf{\Sigma} \\
 &= \mathbf{Tr} \left( \mathbf{Q} \begin{bmatrix} (1 - \frac{1 - \omega_1}{\frac{1}{\alpha} - \omega_1})^2 & & \\ & \ddots & \\ & & (1 - \frac{1 - \omega_N}{\frac{1}{\alpha} - \omega_N})^2 \end{bmatrix} \mathbf{Q}^\top \mathbf{\Sigma} \right). \tag{23}
 \end{aligned}$$

By  $0 \leq \alpha < 1$ , we have  $0 < \frac{1-\omega_i}{\frac{1}{\alpha}-\omega_i} < 1$  for  $1 \leq i \leq N$ . Then, increasing  $\alpha$  will lead to lower variance. Similarly,

$$\begin{aligned}
\text{Bias}(\hat{\mathbf{x}}^*|\hat{\mathbf{x}}, \alpha)^2 &= \mathbb{E} [||\mathbb{E}[\hat{\mathbf{x}}^*] - \hat{\mathbf{x}}||_2^2] \\
&= \mathbb{E} [||\mathbf{H}\hat{\mathbf{x}} - \hat{\mathbf{x}}||_2^2] \\
&= ||(\mathbf{H} - \mathbf{I}_N)\hat{\mathbf{x}}||_2^2 \\
&\approx ||\left(\mathbf{Q} \begin{bmatrix} 1 - \frac{1-\omega_1}{\frac{1}{\alpha}-\omega_1} & & \\ & \ddots & \\ & & 1 - \frac{1-\omega_N}{\frac{1}{\alpha}-\omega_N} \end{bmatrix} \mathbf{Q}^\top - \mathbf{I}_N\right) \hat{\mathbf{x}}||_2^2 \\
&= ||\mathbf{Q} \begin{bmatrix} 1 - \frac{1-\omega_1}{\frac{1}{\alpha}-\omega_1} - 1 & & \\ & \ddots & \\ & & 1 - \frac{1-\omega_N}{\frac{1}{\alpha}-\omega_N} - 1 \end{bmatrix} \mathbf{Q}^\top \hat{\mathbf{x}}||_2^2 \\
&= ||\mathbf{Q} \begin{bmatrix} -\frac{1-\omega_1}{\frac{1}{\alpha}-\omega_1} & & \\ & \ddots & \\ & & -\frac{1-\omega_N}{\frac{1}{\alpha}-\omega_N} \end{bmatrix} \mathbf{Q}^\top \hat{\mathbf{x}}||_2^2 \\
&= ||\mathbf{Q} \begin{bmatrix} \frac{1-\omega_1}{\frac{1}{\alpha}-\omega_1} & & \\ & \ddots & \\ & & \frac{1-\omega_N}{\frac{1}{\alpha}-\omega_N} \end{bmatrix} \mathbf{Q}^\top \hat{\mathbf{x}}||_2^2.
\end{aligned} \tag{24}$$

Therefore, increasing  $\alpha$  will lead to higher bias.  $\square$

## C A Visualization Example Showing that SGCNs are Denoising and Smoothing Node Features

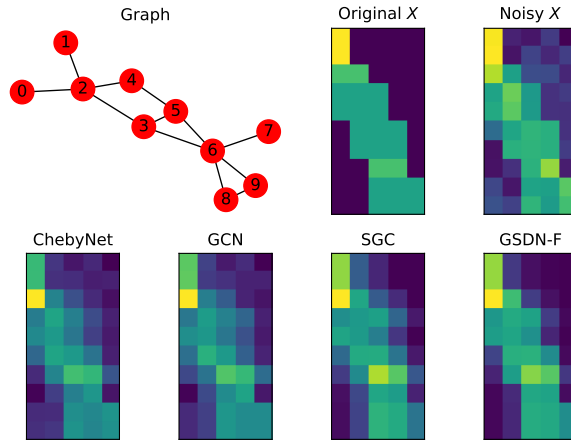

Figure 4: An example of node feature denoising and smoothing by spectral graph convolutions (GSDN-F is introduced in Section 4.1). The original node features are disrupted by the Gaussian noise with  $\mu = 0$  and  $\sigma = 0.01$ . Best viewed in color

Figure 4 shows an example of using spectral graph convolutions to denoise and smooth the node features of a toy graph discussed in Section 3.1. From the figure, we can see SGCNs such as GCN and SGC are not extracting high-level features, but simply denoising and smoothing the noisy node features.

## 68 D Datasets and Experimental Setup

69 **Datasets.** We used Cora, CiteSeer, and Pubmed citation networks (Sen et al., 2008) in the transduc-  
70 tive learning task and the PPI protein-protein interaction network (Zitnik & Leskovec, 2017) in the  
71 inductive learning task. We also conducted experiments by adding noise to node features or edges in  
72 the Cora and CiteSeer datasets to evaluate the performance of GNNs on graphs with noise. Some  
73 information about the datasets are listed in Table 3.

Table 3: Datasets

| Dataset  | #Nodes | #Edges  | Train/Dev/Test     |
|----------|--------|---------|--------------------|
| Cora     | 2,708  | 5,429   | 140/500/1,000      |
| CiteSeer | 3,327  | 4,723   | 120/500/1,000      |
| Pubmed   | 19,717 | 44,338  | 60/500/1,000       |
| PPI      | 56,944 | 818,716 | 44,906/6,514/5,524 |

74 **Baselines.** For the baselines of spectral approaches of GNNs, we compared our models with  
75 ChebyNet (Defferrard et al., 2016), GCN (Kipf & Welling, 2017), and SGC (Wu et al., 2019). For  
76 non-spectral approaches, we chose GraphSage (Hamilton et al., 2017), GAT (Velickovic et al., 2018),  
77 and AGNN (Thekumparampil et al., 2018). We used the released implementations of these baselines  
78 in PyTorch Geometric (Fey & Lenssen, 2019).

79 **Parameter Setting.** We give the parameter setting for our models and baselines in our experiments  
80 here. For GSDN-F and GSDN-EF, we set the learning rate as 0.02,  $L2$  regularization weight as  
81  $5 \times 10^{-4}$  and the polynomial degree  $K$  as 4. In transductive learning tasks, we set the number  
82 of hidden units as 16, the number of layers as 2. We also use two settings for  $\alpha$ , 0.6 and 1.2, for  
83 both GSDN-F and GSDN-EF and denote the models with different  $\alpha$  as **GSDN-F-0.6**, **GSDN-F-1.2**,  
84 **GSDN-EF-0.6**, and **GSDN-EF-1.2**, respectively. For the inductive learning task, we set hidden  
85 number as 256, the number of layers as 3 and  $\alpha$  as 0.6. For ChebyNet and SGC, we used two settings  
86 for  $K$ , 2 and 4, represented as ChebyNet-2, ChebyNet-4, SGC-2, and SGC-4. Other hyperparameters  
87 for ChebyNet, SGC, and other baselines were set by following the settings in (Kipf & Welling, 2017)  
88 and (Velickovic et al., 2018).

## 89 E Additional Experiments

### 90 E.1 Why Renormalization Trick Works

91 We further discuss the effect of the renormalization trick used in GCN. Without the renormalization  
92 trick, the result of the graph convolution of GCN on signal  $\mathbf{x}$ , defined as  $\mathbf{g} \star \mathbf{x} = (\mathbf{I}_N + \mathbf{A}_n)\mathbf{x}$ , is a  
93 first-order polynomial approximation to  $\hat{\mathbf{x}}^*$  of Problem 1 with  $\alpha = 1$ . As a result of  $\alpha = 1$ , it only  
94 intends to smooth node features and overlooks node feature denoising. Therefore, it is easy to be  
95 disrupted by noise. The renormalization trick shrinks  $\alpha$  into  $(0, 1)$  and allows GCN to consider both  
96 node feature smoothing and denoising by

$$\mathbf{g}_{GCN} \star \mathbf{x} = \tilde{\mathbf{D}}^{-1/2}(\mathbf{I}_N + \mathbf{A})\tilde{\mathbf{D}}^{-1/2} \approx \tilde{\mathbf{D}}^{-1} + \mathbf{D}_r \mathbf{A}_n, \quad (25)$$

97 where  $\mathbf{D}_r = \text{diag}(d_1/\tilde{d}_1, \dots, d_N/\tilde{d}_N)$  and  $d_i/\tilde{d}_i \leq 1$ . Thus, it is more robust to the noise. We  
98 empirically validated the effect of the renormalization trick on node feature denoising. The results of  
99 node feature denoising on Cora and CiteSeer with Gaussian noise are shown in Figure 5.

100 As we can see in Figure 5, the noise in denoised node features obtained by  $\mathbf{I} + \mathbf{A}_n$  is not reduced,  
101 indicating that  $\mathbf{I} + \mathbf{A}_n$  does not denoise node features. It validates that  $\mathbf{I} + \mathbf{A}_n$  overlooks node feature  
102 denoising by setting  $\alpha = 1$ . However, Figure 5 shows that  $\tilde{\mathbf{A}}_n$  and  $\tilde{\mathbf{A}}_n^2$  significantly reduce the noise.  
103 It demonstrates that graph convolutions with the renormalization trick are capable to denoise node  
104 features and validates our conclusion in Section 3.1 that the renormalization trick works as it shrinks  
105  $\alpha$  into  $(0, 1)$  and allows GCN to be able to work on node feature denoising.

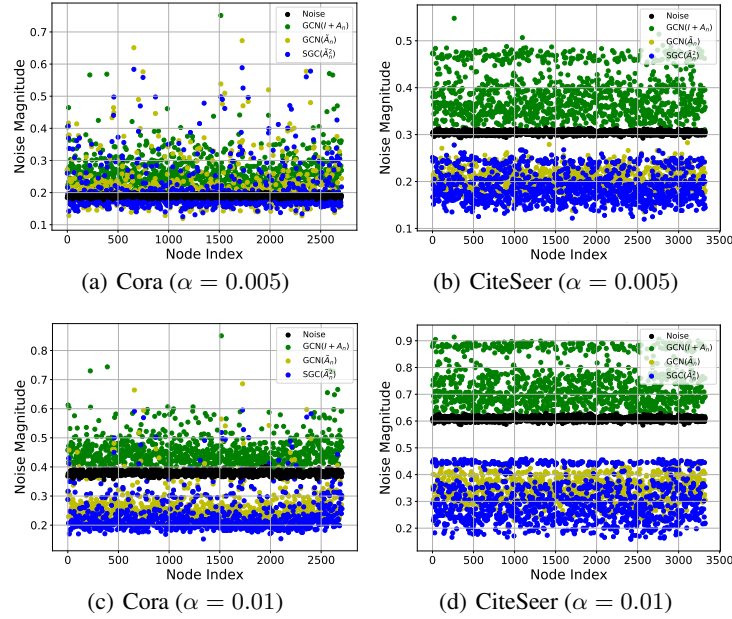

Figure 5: The effect of using the renormalization trick on node feature denoising on graphs with synthetic Gaussian noise ( $\mu = 0$  and  $\sigma = \{0.005, 0.01\}$ ) on node features

## 106 E.2 Experiments on Other Graphs with Noise

107 We conducted experiments on another two datasets, Pubmed and Coauthor CS, using the same  
 108 settings on graphs with noise in Section 5.2. We first normalized the node features and then added  
 109 Gaussian noise with  $\mu = 0$  and  $\sigma = \{0.001, 0.005, 0.01\}$  into the node features, and report the results  
 110 in Figures 6(a) and 6(d). We randomly added or removed edges with noise ratio  $r = \frac{\text{\#noisy edges}}{\text{\#original edges}} =$   
 111  $\{0.05, 0.1, 0.2\}$ , and report the results in Figures 6(b) and 6(e). We also added Gaussian noise into  
 112 node features with  $\mu = 0$  and  $\alpha = \{0.001, 0.005, 0.01\}$  and randomly added or removed edges with  
 113  $r = \{0.05, 0.1, 0.2\}$ , and report the results in Figures 6(c) and 6(f).

114 Figures 6(a) and 6(d) show that the performance of GSDN-F ( $\alpha = 0.6$ ) is better than the other models  
 115 in the noisy node feature cases. The results on Pubmed and Coauthor CS are similar to those on Cora  
 116 and CiteSeer reported in Figures 3(a) and 3(d), which consistently show that GSDN-F ( $\alpha = 0.6$ )  
 117 outperforms GCN and SGC on node classification for graphs with noisy node features.

118 Figures 6(b) and 6(e) show that GSDN-F ( $\alpha = 0.6$ ) also obtained superior performance in the noisy  
 119 edge cases on Pubmed and Coauthor CS. The results validate that GSDN-F ( $\alpha = 0.6$ ) works well in  
 120 the noisy edge cases on Pubmed and Coauthor CS.

121 For graphs with both noisy node features and edges, the results of Figures 6(c) and 6(f) demonstrate  
 122 that GSDN-F ( $\alpha = 0.6$ ) outperforms the models in most cases. Again, GSDN-F ( $\alpha = 0.6$ ) has the  
 123 best performance in the noisy feature and noisy edge cases on Pubmed and Coauthor CS.

124 Thus, the results in Figure 6 demonstrate the effectiveness of GSDN-F on graphs with noisy features  
 125 and/or noisy edges, which is similar with the results obtained on Cora and CiteSeer presented in  
 126 Section 5.2.

## 127 E.3 Parameter Sensitivity Tests

128 In this experiment, we studied the sensitivity of  $\alpha$  and  $K$ . The results are reported in Figure 7.

129 **Variance-bias trade-off by  $\alpha$ .** When  $0 < \alpha \leq 1$ , Figure 7(a) shows that as  $\alpha$  increases, the  
 130 performance of GSDN-F improves first and then dramatically degrades when  $\alpha$  is larger than 0.8.

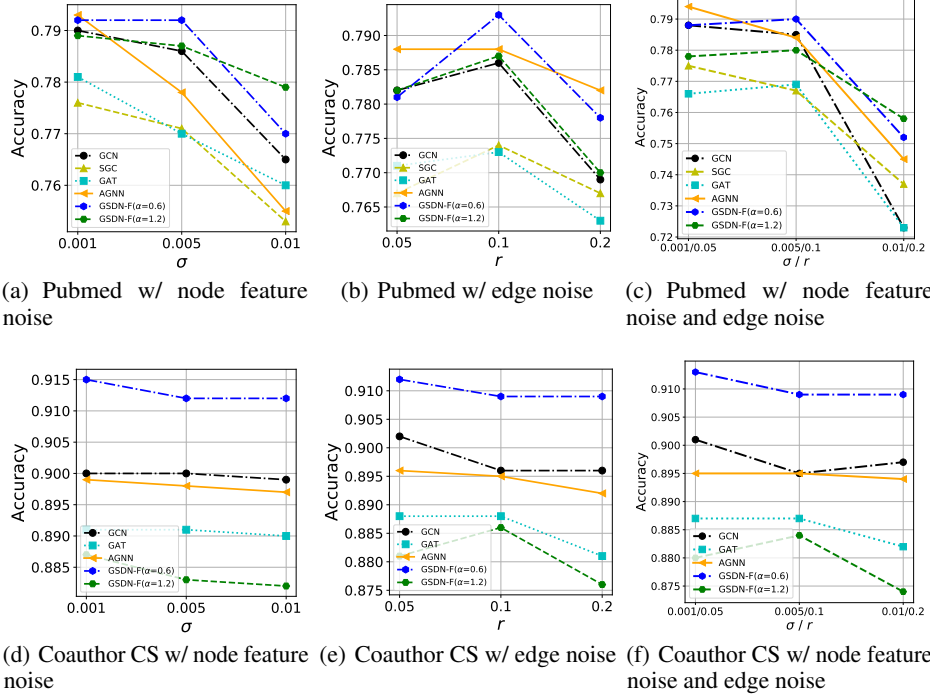

Figure 6: Results of semi-supervised node classification on the Pubmed and Coauthor CS datasets

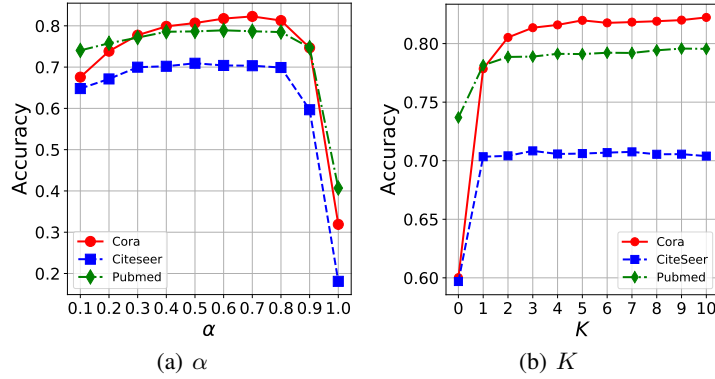

Figure 7: Results of parameter sensitivity

131 The result illustrates that the choice of  $\alpha$  can seriously affect the performance of node classification  
 132 and validates the variance-bias trade-off by  $\alpha$  as stated in Proposition 3.

133 **The effect of polynomial approximation order  $K$ .** Figure 7(b) shows that the performance of  
 134 GSDN-F improves as  $K$  increases and then becomes stable when  $K$  is large enough. This is because  
 135 the larger the value of  $K$  is, the more accurate is the approximation and hence the better performance  
 136 of GSDN-F is.

137 **Parameter Sensitivity for  $\alpha > 1$ .** Here we study the sensitivity of  $\alpha$  for  $\alpha > 1$ . We conducted the  
 138 experiments for semi-supervised node classification on Cora, CiteSeer, and Pubmed with and without  
 139 Gaussian noise ( $\mu = 0, \sigma = 0.01$ ). The results are reported in Figure 8.

140 When  $\alpha > 1$ , Figure 8 shows that as  $\alpha$  increases, the performance of GSDN-F dramatically improves  
 141 first and slightly degrades when  $\alpha$  is larger than 1.2 on both the original graphs and the graphs with

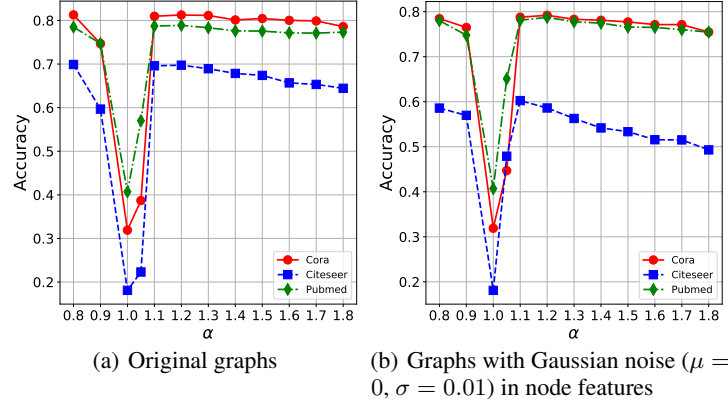

Figure 8: Results of parameter sensitivity of  $\alpha$  for  $\alpha > 1$

142 Gaussian noise in node features. The results suggest that choosing GSDN-F with  $\alpha$  around 1.2 can  
 143 obtain good performance for graphs with a lot of noise.

## 144 References

- 145 Berger, P., Hannak, G., and Matz, G. Graph signal recovery via primal-dual algorithms for total  
 146 variation minimization. *J. Sel. Topics Signal Processing*, 11(6):842–855, 2017.
- 147 Chen, S., Sandryhaila, A., Moura, J. M. F., and Kovacevic, J. Signal recovery on graphs: Variation  
 148 minimization. *IEEE Trans. Signal Processing*, 63(17):4609–4624, 2015.
- 149 Defferrard, M., Bresson, X., and Vandergheynst, P. Convolutional neural networks on graphs with  
 150 fast localized spectral filtering. In *Advances in Neural Information Processing Systems 29: Annual  
 151 Conference on Neural Information Processing Systems, December 5-10, 2016, Barcelona, Spain*,  
 152 pp. 3837–3845, 2016.
- 153 Fey, M. and Lenssen, J. E. Fast graph representation learning with PyTorch Geometric. In *7th  
 154 International Conference on Learning Representations, New Orleans, LA, USA, May 6-9, 2019,  
 155 Workshop on Representation Learning on Graphs and Manifolds*, 2019.
- 156 Hamilton, W. L., Ying, Z., and Leskovec, J. Inductive representation learning on large graphs. In  
 157 *Advances in Neural Information Processing Systems 30: Annual Conference on Neural Information  
 158 Processing Systems, 4-9 December 2017, Long Beach, CA, USA*, pp. 1024–1034, 2017.
- 159 Hammond, D. K., Vandergheynst, P., and Gribonval, R. Wavelets on graphs via spectral graph theory.  
 160 *Applied and Computational Harmonic Analysis*, 30(2):129–150, 2011.
- 161 Henaff, M., Bruna, J., and LeCun, Y. Deep convolutional networks on graph-structured data. *CoRR*,  
 162 abs/1506.05163, 2015.
- 163 Kipf, T. N. and Welling, M. Semi-supervised classification with graph convolutional networks. In  
 164 *5th International Conference on Learning Representations, Toulon, France, April 24-26, 2017,  
 165 Conference Track Proceedings*, 2017.
- 166 Sandryhaila, A. and Moura, J. M. F. Discrete signal processing on graphs. *IEEE Trans. Signal  
 167 Processing*, 61(7):1644–1656, 2013.
- 168 Sen, P., Namata, G., Bilgic, M., Getoor, L., Gallagher, B., and Eliassi-Rad, T. Collective classification  
 169 in network data. *AI Magazine*, 29(3):93–106, 2008.
- 170 Thekumparampil, K. K., Wang, C., Oh, S., and Li, L. Attention-based graph neural network for  
 171 semi-supervised learning. *CoRR*, abs/1803.03735, 2018.



- 172 Velickovic, P., Cucurull, G., Casanova, A., Romero, A., Liò, P., and Bengio, Y. Graph attention  
173 networks. In *6th International Conference on Learning Representations, Vancouver, BC, Canada,*  
174 *April 30 - May 3, 2018, Conference Track Proceedings*, 2018.
- 175 Wu, F., Jr., A. H. S., Zhang, T., Fifty, C., Yu, T., and Weinberger, K. Q. Simplifying graph  
176 convolutional networks. In *Proceedings of the 36th International Conference on Machine Learning,*  
177 *9-15 June 2019, Long Beach, California, USA*, pp. 6861–6871, 2019.
- 178 Zitnik, M. and Leskovec, J. Predicting multicellular function through multi-layer tissue networks.  
179 *Bioinformatics*, 33(14):190–198, 2017.
